# Supplementary material for: Disentangling Internal Tides from Balanced Motions with Deep Learning and Surface Field Synergy
Source: arXiv:2511.03614 ancillary file (2026-04-27)
Supplement: Supplementary file 1 [file Supporting_Information.pdf]

# Supporting Information for “Disentangling Internal Tides from Balanced Motions with Deep Learning and Surface Field Synergy”

Han Wang<sup>1</sup>, Jeffrey Uncu<sup>2</sup>, Kaushik Srinivasan<sup>3</sup>, Nicolas Grisouard<sup>2</sup>

<sup>1</sup>Institute of Oceanography, University of Hamburg, 20146 Hamburg, Germany

<sup>2</sup>Department of Physics, University of Toronto, Toronto ON M5S 1A7, Canada

<sup>3</sup>University of California, Los Angeles, CA 90095, USA

## Contents of this file

1. Text S1 to S5
2. Figures S1 to S2
3. Tables S1 to S2

## Text S1: Details on the deep learning algorithm

This section documents the U-Net’s model implementation and hyperparameter choices for reproducibility. For brevity, we assume readers of this section are familiar with concepts in neural network architectures and do not explain some related standard terminologies.

Our codes for the U-Net architecture are modified from a Github implementation <https://github.com/milesial/Pytorch-UNet>, commit 21d7850) and are available at Wang (2025). Our choices of hyperparameters, such as the overall sizes of the U-Net, are

all determined empirically with Configuration  $\{H\}$ . For example, we vary the size of the U-Net under the Configuration  $\{H\}$ , and find out that the performances are not affected if the number of kernels are reduced to one quarter of the number used by Ronneberger, Fischer, and Brox (2015); cutting the kernel number by a further half would slightly decrease the performance. This led us to decide to keep the number of kernels to be as described in the main text.

In the spirit of minimizing computational resources, we also maximize the batch sizes of training data to better parallelize the computations on the GPUs. We choose the largest batch sizes that can fit into our GPU's typical memory (40 GB), and, for ease of batch allocation, be divisible by the number of total number of snapshots in the training data (600). The batch sizes for inputs with 1, 2, 3, and 4 channels are taken to be 100, 80, 60 and 50 respectively. In principle, having large batch sizes may introduce issues for the generalization performance, as the parameter updates may not be refined enough (Clevert et al., 2015). As a precautionary check against this, we experimented on Configuration  $\{H\}$  with batch sizes of 10 and batch sizes of 100, and did not find significant differences in the performances metrics.

Our U-Net is much faster to train than the cGAN in W22. As an illustration, one author ran our U-Net and the cGAN in W22 for the Configuration  $\{H\}$  on an Nvidia 3070 GPU. GPUs of this capacity are frequently found on portable computers. On this GPU, for 300 epochs, it takes 18 hours to train the cGAN, and just 1 hour to train our U-Net. This difference in computational costs could be narrowed if we optimize the computational efficiency of the cGAN, but the complicated architecture and relatively unstable training behavior of cGANs makes this challenging. The main bottleneck that affects the training

time of our U-Net is in data loading. At each epoch, it takes more time to load training data to the GPU than to conduct the optimization procedures. In future, if we are to further cut down training time, the data loading efficiency would be the first to target.

In our application, different physical fields have different overall magnitudes; for example, the variances of raw SSH and IT SSH differ by an order of  $10^5$ . Data normalization is conducted to facilitate the training’s convergence (LeCun et al., 2002). Prior to training, we shift and rescale the data so that data from each input or output channel has a zero mean and variance of 1 over the entire set (including training and testing sets), as also done in W22.

In principle, the normalization can also be included as part of the neural network’s architecture via batch normalization layers, which some would argue can accelerate convergence and enhance model generalization (Ioffe, 2015). However, we find that in our applications, batch-normalization layers, once combined with large batch sizes, destroy the stability of training behaviors as shown in Text S2 for the U-Net without built-in batch-normalization layers; the U-Net’s performance metrics would be dramatically different (often differing by a more than factor of 2 in mean  $R_2$ ) each time we re-initialize and re-train it under the same configuration when the batch sizes are 50. When the batch sizes are small (at, say, 10), the trained U-Nets are stable, but generates spurious features at scales below the mode-1 IT wavelength, suggesting that the U-Net learns false connections and hallucinates features; this behavior disappears if we delete the batch normalization layers and scale the data prior to training, as we eventually choose to do.

During training, the learning rate changes periodically with respect to number of epochs. For every configuration, we train the U-Net for 300 epochs, and save the checkpoints at

the epoch where the trained model achieves the highest  $R_2$  averaged over all the testing data. This practice of saving the best model (as opposed to, say, saving the model at a fixed epoch) is common when learning rate changes (Loshchilov & Hutter, 2016).

The specific scheme we apply for the learning rate follows (Liu, 2022), prescribed as

$$\text{lr} = \frac{1}{2}\eta_{\max} \left( 1 + \cos \left( \frac{\text{epoch} - t_i}{T_0} \pi \right) \right), \quad (1)$$

where “lr” is the learning rate,  $\eta_{\max}$  is the maximum learning rate set as 0.05 divided by the batch size, “epoch” is the epoch number,  $T_0$  is the period of the learning rate set as 10 epochs, and

$$t_i = (\text{epoch} // T_0) T_0, \quad (2)$$

where “//” denotes floor division. Within each period  $T_0$ , the learning rate starts at  $\eta_{\max}$  and decays like a cosine function (at the range between 0 and  $\pi$ ) with a gradual decrease to 0. At the start of the next period, the learning rate abruptly jumps back to  $\eta_{\max}$ .

In addition to (1), we have experimented with another annealing scheme taken from (Smith, 2017), prescribed as

$$\text{lr} = \eta_{\max} \text{Max} [0, 1 - |2\text{epoch}/T_0 - 2(1 + \text{epoch} // T_0) + 1|], \quad (3)$$

where  $\text{Max}[a, b]$  denotes taking the larger values between  $a$  and  $b$ , and  $|\cdot|$  denotes taking the absolute value. Under scheme (3), within each cycle with period  $T_0$ , the learning rate increases linearly from 0 to  $\eta_{\max}$  over the first half of the period, and then decreases linearly back to 0 for the second half of the period. For  $T_0$ , we experimented with 10 or 20 epochs for this scheme. Figure S1 illustrates that changing from scheme (1) (lines with legend label “Tcycle10”) to scheme (3) (lines with legend labels starting with “tri”), or increasing  $T_0$  from 10 (lines with legend label “tri5”) to 20 (lines with legend label “tri10”)

epochs, does not affect the performance of Configuration  $\{H\}$  once the trainings converge: the corresponding lines (last three in the line legend label) in Figure S1 converge to nearly identical mean  $R_2$  coefficients at large epochs. Therefore, the performance of our U-Net does not appear sensitive to changes in the specifics of the learning rate annealing scheme.

What does affect the performance significantly is the existence of a non-constant learning rate. As explained in the main text, a non-constant learning rate encourages the optimizer to escape local minima while still preserving accuracy and convergence. In Figure S1, we show that larger constant learning rates (fourth line in the line legends) do not make the U-Net to converge at all, while under smaller constant learning rates (first three lines in the line legends), the U-Net does converge, but to states where the mean  $R_2$  are significantly lower than the mean  $R_2$  produced by U-Nets trained by periodically changing learning rates (last three lines in the line legends); this is consistent with our understanding that when learning rates are too small, the U-Nets stop optimizing after local minima are reached, missing the global minima.

All data from our Boussinesq simulations are originally formatted to be of sizes 258-by-722, with grid spacing of 4 km. We crop the outmost grid points, so that the images have 256 and 720 grid points in the longitudinal and latitudinal direction. The cropped images have number of grid points divisible by  $2^4$ , which circumvents padding issues in the U-Net architecture. All training images are rectangular with this size. As the network is fully convolutional, once trained, it can be directly applied to images of any aspect ratios, lengths or widths, as long as the grid spacing is kept the same.

In W22, the output of the deep learning model was  $h_{\cos}^{\text{sim}}$  only, while here we include both  $h_{\cos}^{\text{sim}}$  and  $h_{\sin}^{\text{sim}}$  in the outputs. Learning both Fourier coefficients is more useful than learning

just  $h_{\cos}^{\text{sim}}$  because with both the Fourier coefficients, one can in principle reconstruct the IT time series locally in time. Moreover,  $h_{\cos}^{\text{sim}}$  and  $h_{\sin}^{\text{sim}}$  are not independent, as they are fingerprints from the same dynamical field; adding dependent outputs to a deep learning model could improve the performance, as the model can leverage shared features between these outputs (Caruana, 1997). In our application, we find out that including both  $h_{\cos}^{\text{sim}}$  and  $h_{\sin}^{\text{sim}}$  indeed slightly improves the performances (details not shown).

We use the  $L_1$  loss as the only term in the training loss function. Compared to training loss functions of higher orders (such as the  $L_2$  loss), the model is penalized less when producing the average of a given field. We do not find significant differences between using a  $L_1$  and a  $L_2$  loss. In future works, we will explore the impacts from different forms of training loss functions, particularly in the context of fixing error at small spatial scales.

## **Text S2: Stability of training behaviors**

For each configuration, we re-initialize and re-train the U-Net for 10 times. As the initial kernel values are assigned with different random numbers, the 10 U-Nets can be in principle different between each other, even though their architecture and configurations are the same. The point of the re-initialization and the subsequent analysis described here is to investigate the sensitivity of the performances to different random initial values.

For each re-trained 10 U-Net, we compute the  $\Upsilon$  in the testing data, averaged over the full simulation domain (marked as “full” in the first column of Table S1) or the mid-jet region (marked as “mid” in the first column of Table S1). Table S1 (second - fifth columns) show the mean, maximum, minimum and standard deviations of the 10 values

of  $\Upsilon$  under each configuration averaged over the full or mid-jet regions in the testing data separately. Table S2 shows the corresponding behaviours of  $R_2$ .

In the main text, for brevity, we show the performances from one (randomly chosen and fixed) of the ten re-trained U-Nets under each configuration. In terms of either  $\Upsilon$  or  $R_2$ , and over either mid-jet or the full regions averaged over the testing data set, the performances of the configurations described in the main text can be ordered from low-performing to high-performing as:

$$\{T\} < \{H\} < \{H, T\} < \{U\} < \{U, T\} < \{H, U\} < \{H, U, T\} \quad (4)$$

This ordering also holds for  $\Upsilon$  and  $R_2$  in the mean, maximum, and minimum for full and mid-jet regions shown in Tables S1 and S2. This reassures us that when one configuration performs better than the other, the improvement is unambiguous.

From Tables S1 and S2, the standard deviation of  $\Upsilon$  is at most 0.022, and the standard deviation of  $R_2$  is at most 0.026. Thus, when a U-Net has a  $\Upsilon$  or  $R_2$  value higher than another U-Net by more than 0.1, which comfortably exceeds three times the standard deviations, the former U-Net's higher performance is unlikely caused by random fluctuations from training. As the differences between different configurations in the main text exceed 0.1, we can also be reassured that the differences exceed the statistical uncertainty associated with random initializations.

### **Text S3: Configurations $\{U\}$ and $\{V\}$**

Configurations  $\{U\}$  and  $\{V\}$  are run with only one velocity component in  $\mathbf{U} = (U, V)$  as the input. As with other configurations, we re-train the U-Nets for 10 times each, and record the statistics in Table S1 and S2. They both appear stable, showing little deviations between each re-train. The mean, maximum and minimum of  $\Upsilon$  and  $R_2$  computed over

the mid-jet or full regions from the Configurations  $\{U\}$  and  $\{V\}$  are all higher than the counterparts from the Configurations  $\{H\}$  and  $\{T\}$ , demonstrating an unambiguously better performance from the Configurations  $\{U\}$  and  $\{V\}$ .

This implies that the information contained in a single velocity component is more useful than the information contained in  $\{H\}$  or  $\{T\}$  alone. The performances of Configurations  $\{U\}$  and  $\{V\}$  are different between each other; this is not surprising, as several aspects of our simulations (e.g., IT forcing, background density profile) are not set up to be horizontally isotropic.

#### **Text S4: Configurations with smoothed $T$ as inputs**

We convolve  $T$  in the  $(x, y)$  space with a normalized Gaussian kernel whose full width at half maximum (hereafter “FWHM”) is 20 km or 100 km. These are equivalent to multiplying the images with Gaussian decay functions in the wavenumber space; the images are thus low-pass filtered. We regard the wavelength at which the data are cut to 10% of its original value as the effective resolution. This effective resolution is 25 km and 124 km for the Gaussian kernels with FWHMs at 20 km and 100 km respectively. We denote the resulting low-pass filtered fields as  $\bar{T}^{25}$  and  $\bar{T}^{124}$ , where the superscripts refer to the effective resolutions. Figure S2 shows a snapshot of  $T$ ,  $\bar{T}^{25}$ , and  $\bar{T}^{124}$ .

We study the effects of this smoothing on Configurations  $\{H, T\}$ ,  $\{U, T\}$  and  $\{H, U, T\}$ , replacing  $T$  with  $\bar{T}^{25}$  or  $\bar{T}^{124}$ . As explained in the main text, Configuration  $\{T\}$  generates no meaningful outputs when the ITs are incoherent, and is therefore not analyzed further here. Similar to other configurations, each configuration involving  $\bar{T}^{25}$  or  $\bar{T}^{124}$  is re-trained for 10 times, and the statistics of  $\Upsilon$  and  $R_2$  are recorded in Table S1 and Table S2. The mean, maximum, and minimum of  $\Upsilon$  or  $R_2$  over full or mid-jet regions improve in tandem

between configurations, therefore, for brevity, we only discuss the  $\Upsilon$  over the mid-jet regions (shaded rows of Table S1).

The difference in the mean mid-jet  $\Upsilon$  (second column of Table S1) between Configurations  $\{H, T\}$  and  $\{H, \bar{T}^{25}\}$  is less than 0.01. This difference is already at a similar magnitude to the standard deviation (last column), suggesting that the marginal improvement we see of Configuration  $\{H, T\}$  over  $\{H, \bar{T}^{25}\}$  in terms of mean  $\Upsilon$  could be overwhelmed by the small statistical fluctuations. Indeed, the maximum of mid-jet  $\Upsilon$  (third column) in Configuration  $\{H, \bar{T}^{25}\}$  is higher than the minimum of mid-jet  $\Upsilon$  (fourth column) in Configuration  $\{H, T\}$ , meaning that among the 10 re-trained U-Nets from each configuration, one can pick a U-Net from the Configuration  $\{H, \bar{T}^{25}\}$  that outperforms a U-Net from the Configuration  $\{H, T\}$ . The same can be said for the differences between Configurations  $\{U, T\}$  and  $\{U, \bar{T}^{25}\}$ , or between Configurations  $\{H, U, T\}$  and  $\{H, U, \bar{T}^{25}\}$ . Therefore, smoothing  $T$  to  $\bar{T}^{25}$  does not affect the performances in a statistically meaningful way.

From Table S1, the mean mid-jet  $\Upsilon$  of Configuration  $\{H, \bar{T}^{124}\}$  is lower than the mid-jet  $\Upsilon$  of Configuration  $\{H, T\}$  by 0.029. This is a small decrease, but statistically significant in the sense that it is much larger than the standard deviations; similarly, unlike the case of  $\{H, T\}$  and  $\{H, \bar{T}^{25}\}$ , the minimum of  $\Upsilon$  from the Configuration  $\{H, T\}$  is higher than the maximum of  $\Upsilon$  from the Configuration  $\{H, \bar{T}^{124}\}$ . The same statement can be made for the difference between Configuration  $\{U, \bar{T}^{124}\}$  and Configuration  $\{U, T\}$ . However, the difference between Configuration  $\{H, U, \bar{T}^{124}\}$  and Configuration  $\{H, U, T\}$  is too small to be statistically significant, as the differences in the means are comparable to the standard deviations. Therefore, smoothing  $T$  to  $\bar{T}^{124}$  slightly decreases the performances

of Configurations  $\{H, T\}$  and  $\{U, T\}$ , while not affecting the performance of Configuration  $\{H, U, T\}$  in a statistically meaningful way.

For a more thorough inspection, we also compare the wavenumber spectra from the Configurations  $\{H, U, T\}$ ,  $\{H, U, \bar{T}^{25}\}$  and  $\{H, U, \bar{T}^{124}\}$  (Figure S3). In the down-jet region, some small differences can be seen between Configurations  $\{H, U, T\}$  and  $\{H, U, \bar{T}^{124}\}$  at wavenumber higher than the mode-1 wavenumbers, while otherwise, the differences are barely perceptible.

Although Configuration  $\{H, \bar{T}^{124}\}$  performs slightly worse than Configuration  $\{H, T\}$ , it still outperforms Configuration  $\{H\}$  significantly (0.08 in mean mid-jet  $\Upsilon$ ). In other words, although some useful information in  $T$  is lost after the relatively aggressive smoothing, the loss is small, and having the smoothed  $\bar{T}^{124}$  is still significantly better than not having it in the inputs.

#### **Text S5: Configurations with vorticity and/or divergence as inputs**

We are not aware of observational instruments that can accurately measure surface vorticity  $\zeta$  and surface divergence  $D$  in the ocean, and our experiments with them are motivated purely by theoretical curiosities about the impacts of wave signature versus scattering medium on the performance; as explained in the main text, in our simulation data,  $D$  mainly contains mainly only wave imprints, while  $\zeta$  contains imprints from both waves and BMs.

We re-train each configuration for 4 times and have confirmed that the outputs are stable at each re-train, provided that the U-Net’s hyperparameters (e.g., batch size) are the same. For brevity, we only discuss the mean  $\Upsilon$  or  $R_2$  averaged over the full simulation domain in the testing set, generated from one of the 4 re-trained U-Nets.

Some problematic behaviors are found in Configuration  $\{\zeta\}$ : when some hyperparameters are different, the results are inconsistent. The mean  $\Upsilon$  is 0.82 if we keep all the U-Net’s hyperparameters to be exactly the same as our main U-Net (Supporting Information Text S1); in particular, the batch size would be 100. However, if we decrease the batch size to 10, the mean  $\Upsilon$  increases to 0.86, which is beyond the fluctuations between re-trained models. Thus, the batch size affects the performance of Configuration  $\{\zeta\}$  significantly.

Another confounding behavior is shown when we experiment changing the output field to be just  $h_{\cos}^{\text{sim}}$ . Under other configurations of input fields, when the output field contains both  $h_{\cos}^{\text{sim}}$  and  $h_{\sin}^{\text{sim}}$ , the performance increases, which has a heuristic explanation from multi-task learning, as explained in the Supporting Information Text S1; thus, outside this section, we only discuss the performances of experiments with both  $h_{\cos}^{\text{sim}}$  and  $h_{\sin}^{\text{sim}}$  in the outputs. However, the performance of Configuration  $\{\zeta\}$  is better when the output field contains only  $h_{\cos}^{\text{sim}}$ , which is counter-intuitive.

Due to these problematic behaviors, we refrain from drawing any further conclusions about Configuration  $\{\zeta\}$ . The information contained in  $\zeta$  may be difficult for the current U-Net architecture to exploit effectively. To revisit this, an in-depth investigation into the design of the machine learning algorithm is required.

We do not find such problematic behaviors in any other configurations discussed in this work.

Configuration  $\{D\}$  gives a mean  $\Upsilon$  of 0.88. This outperforms all the other configurations with only one input channel, including Configurations  $\{U\}$  or  $\{V\}$  (detailed in Supporting Information Text S3).

We also experiment with Configuration  $\{\zeta, D\}$ , which takes both vorticity and divergence as inputs. The mean  $\Upsilon$  and  $R_2$  are 0.93 and 0.86 respectively, which are slightly (but significantly) worse than the mean  $\Upsilon$  and  $R_2$  found in Configuration  $\{\mathbf{U}\}$  (0.94 and 0.88).

## References

- Caruana, R. (1997). Multitask learning. *Machine learning*, 28, 41–75.
- Clevert, D.-A., Unterthiner, T., & Hochreiter, S. (2015). Fast and accurate deep network learning by exponential linear units (elus). *arXiv preprint arXiv:1511.07289*.
- Ioffe, S. (2015). Batch normalization: Accelerating deep network training by reducing internal covariate shift. *arXiv preprint arXiv:1502.03167*.
- LeCun, Y., Bottou, L., Orr, G. B., & Müller, K.-R. (2002). Efficient backprop. In *Neural networks: Tricks of the trade* (pp. 9–50). Springer.
- Liu, Z. (2022). Super convergence cosine annealing with warm-up learning rate. In *Caibda 2022; 2nd international conference on artificial intelligence, big data and algorithms* (pp. 1–7).
- Loshchilov, I., & Hutter, F. (2016). Sgdr: Stochastic gradient descent with warm restarts. *arXiv preprint arXiv:1608.03983*.
- Ronneberger, O., Fischer, P., & Brox, T. (2015). U-net: Convolutional networks for biomedical image segmentation. In *Medical image computing and computer-assisted intervention—miccai 2015: 18th international conference, munich, germany, october 5-9, 2015, proceedings, part iii 18* (pp. 234–241).
- Smith, L. N. (2017). Cyclical learning rates for training neural networks. In *2017 IEEE winter conference on applications of computer vision (wacv)* (pp. 464–472).

Wang, H. (2025, November). *hannnwang/extract\_internal\_tides\_with\_unet\_and\_surface\_field\_synergy: For zenodo*. Zenodo. Retrieved from <https://doi.org/10.5281/zenodo.17525907> doi: 10.5281/zenodo.17525907

**Table S1.** The mean, maximum, minimum and stand deviations of the 10 values of mean  $\Upsilon$  from the re-trained U-Net under each configuration, averaged over the full or mid-jet regions in the testing data separately. To make small differences visible,  $\Upsilon$  are rounded up to the fourth digit after zero, containing two more digits than  $\Upsilon$  listed in the main text.

| Configuration, region                     | Mean   | Maximum | Minimum | Standard deviation |
|-------------------------------------------|--------|---------|---------|--------------------|
| $\{H\}$ , full                            | 0.7908 | 0.7964  | 0.7868  | 0.0029             |
| $\{H\}$ , mid                             | 0.6781 | 0.6872  | 0.6689  | 0.0059             |
| $\{H, \mathbf{U}, T\}$ , full             | 0.9708 | 0.9763  | 0.9515  | 0.0077             |
| $\{H, \mathbf{U}, T\}$ , mid              | 0.9531 | 0.9629  | 0.9202  | 0.0132             |
| $\{T\}$ , full                            | 0.3970 | 0.4168  | 0.3700  | 0.0143             |
| $\{T\}$ , mid                             | 0.0442 | 0.0697  | 0.0066  | 0.0222             |
| $\{\mathbf{U}\}$ , full                   | 0.9407 | 0.9415  | 0.9400  | 0.0006             |
| $\{\mathbf{U}\}$ , mid                    | 0.9021 | 0.9038  | 0.8996  | 0.0012             |
| $\{H, T\}$ , full                         | 0.8568 | 0.8619  | 0.8488  | 0.0038             |
| $\{H, T\}$ , mid                          | 0.7902 | 0.8015  | 0.7783  | 0.0067             |
| $\{H, \mathbf{U}\}$ , full                | 0.9627 | 0.9744  | 0.9529  | 0.0079             |
| $\{H, \mathbf{U}\}$ , mid                 | 0.9384 | 0.9594  | 0.9218  | 0.0141             |
| $\{\mathbf{U}, T\}$ , full                | 0.9522 | 0.9534  | 0.9507  | 0.0008             |
| $\{\mathbf{U}, T\}$ , mid                 | 0.9198 | 0.9217  | 0.9178  | 0.0014             |
| $\{U\}$ , full                            | 0.8151 | 0.8189  | 0.8090  | 0.0027             |
| $\{U\}$ , mid                             | 0.6946 | 0.7030  | 0.6847  | 0.0052             |
| $\{V\}$ , full                            | 0.8560 | 0.8579  | 0.8542  | 0.0011             |
| $\{V\}$ , mid                             | 0.7768 | 0.7798  | 0.7740  | 0.0019             |
| $\{H, \bar{T}^{25}\}$ , full              | 0.8556 | 0.8628  | 0.8486  | 0.0042             |
| $\{H, \bar{T}^{25}\}$ , mid               | 0.7897 | 0.8012  | 0.7788  | 0.0068             |
| $\{H, \bar{T}^{124}\}$ , full             | 0.8394 | 0.8432  | 0.8341  | 0.0028             |
| $\{H, \bar{T}^{124}\}$ , mid              | 0.7616 | 0.7676  | 0.7521  | 0.0053             |
| $\{\mathbf{U}, \bar{T}^{25}\}$ , full     | 0.9514 | 0.9528  | 0.9492  | 0.0010             |
| $\{\mathbf{U}, \bar{T}^{25}\}$ , mid      | 0.9183 | 0.9208  | 0.9151  | 0.0017             |
| $\{\mathbf{U}, \bar{T}^{124}\}$ , full    | 0.9456 | 0.9464  | 0.9442  | 0.0006             |
| $\{\mathbf{U}, \bar{T}^{124}\}$ , mid     | 0.9083 | 0.9093  | 0.9057  | 0.0010             |
| $\{H, \mathbf{U}, \bar{T}^{25}\}$ , full  | 0.9671 | 0.9738  | 0.9604  | 0.0042             |
| $\{H, \mathbf{U}, \bar{T}^{25}\}$ , mid   | 0.9471 | 0.9587  | 0.9349  | 0.0075             |
| $\{H, \mathbf{U}, \bar{T}^{124}\}$ , full | 0.9653 | 0.9738  | 0.9510  | 0.0081             |
| $\{H, \mathbf{U}, \bar{T}^{124}\}$ , mid  | 0.9438 | 0.9589  | 0.9194  | 0.0138             |

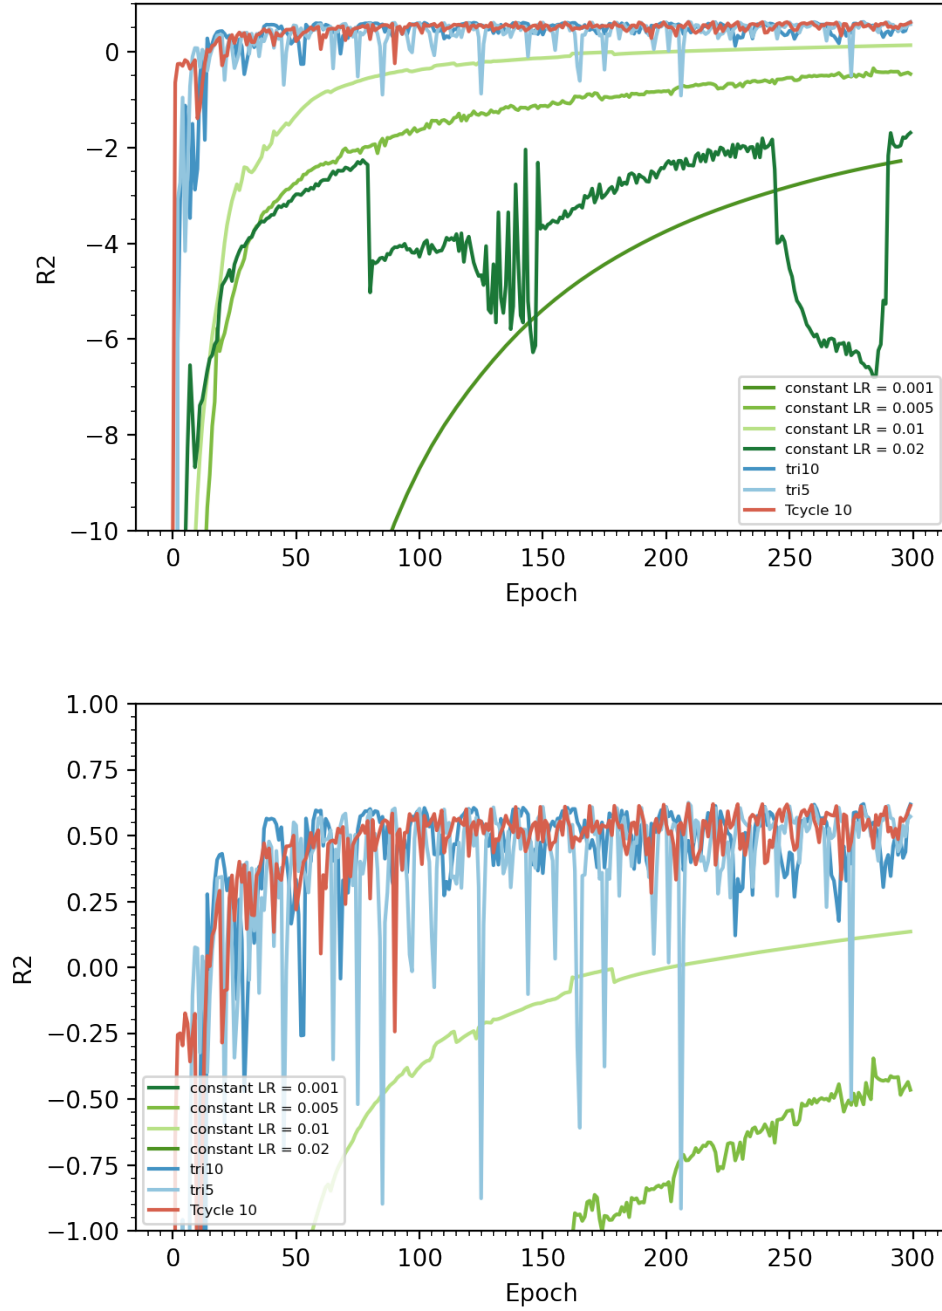

**Figure S1.** Impacts of different learning rate schemes on the U-Net's performance in Configuration  $\{H\}$ . Horizontal axis is the epoch number, and vertical axis is the mean  $R_2$  (averaged over full simulation domain in the testing data) between the reference and the fields generated by the U-Net trained right after the corresponding epoch has passed. The lower panel is a zoomed-in plot of the upper panel.

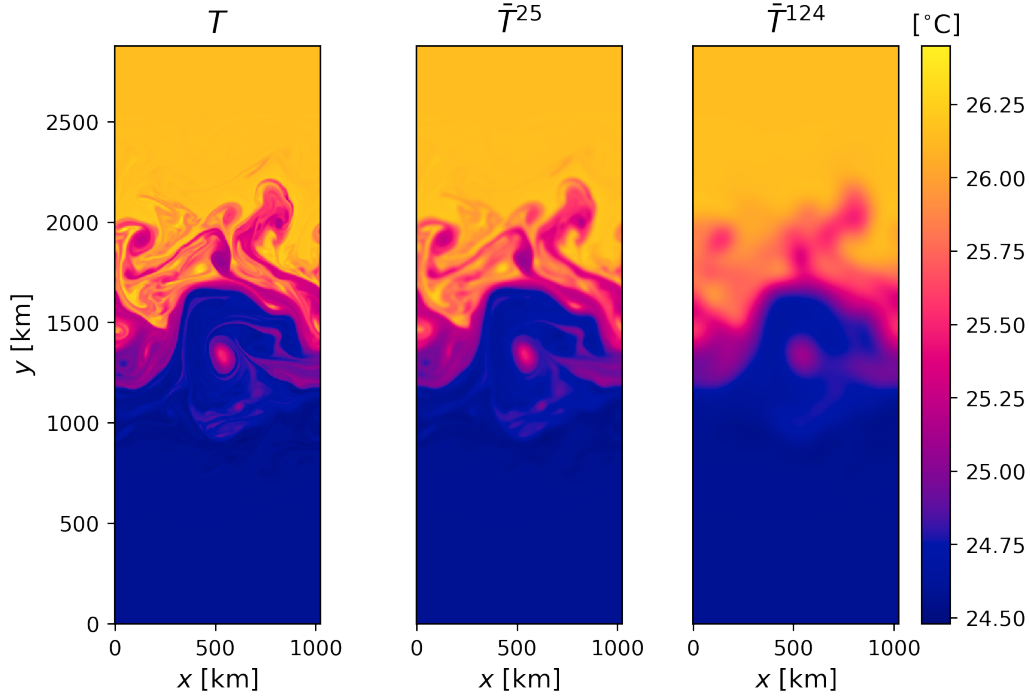

**Figure S2.** Snapshot of  $T$  (first panel),  $\bar{T}^{25}$  (second panel) and  $\bar{T}^{124}$  (third panel). Plotted at the same T5 snapshot as in Figure 1 in the main text.

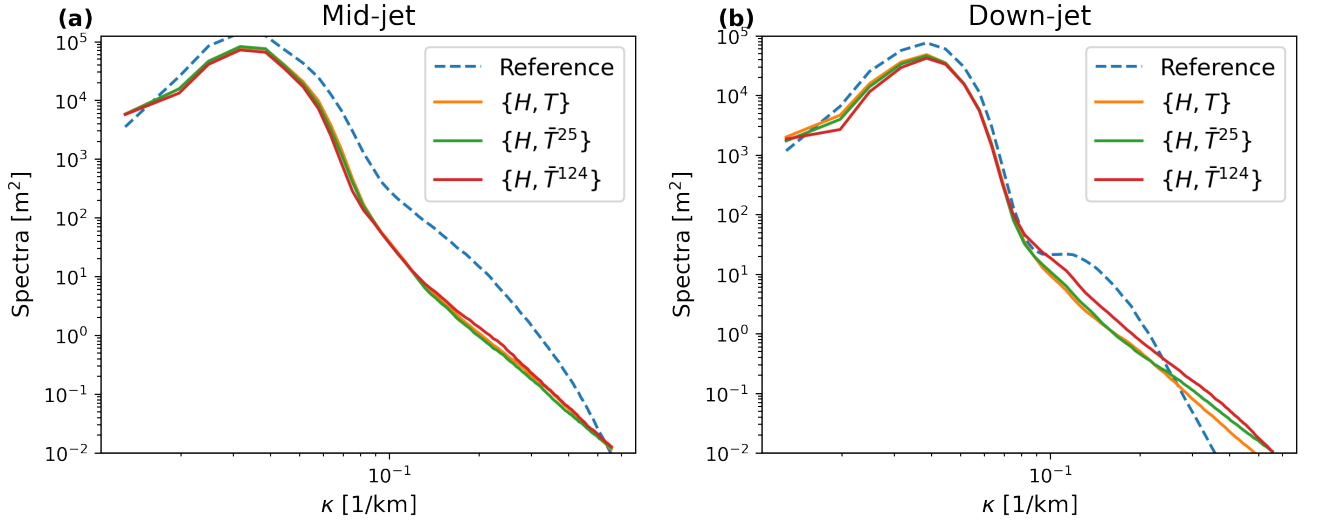

**Figure S3.** Comparison of wavenumber spectra of Configuration  $\{H, T\}$  before and after smoothing  $T$ ; plotting setups are similar to Figure 9 in the main text. )

**Table S2.** Similar to Table S1, but for  $R_2$  instead of  $\Upsilon$ .

| Configuration, region                     | Mean    | Maximum | Minimum | Standard deviation |
|-------------------------------------------|---------|---------|---------|--------------------|
| $\{H\}$ , full                            | 0.6235  | 0.6338  | 0.6175  | 0.0046             |
| $\{H\}$ , mid                             | 0.4544  | 0.4689  | 0.4431  | 0.0078             |
| $\{H, \mathbf{U}, T\}$ , full             | 0.9421  | 0.9528  | 0.9052  | 0.0148             |
| $\{H, \mathbf{U}, T\}$ , mid              | 0.9078  | 0.9264  | 0.8467  | 0.0248             |
| $\{T\}$ , full                            | 0.1453  | 0.1649  | 0.1227  | 0.0137             |
| $\{T\}$ , mid                             | -0.0491 | -0.0156 | -0.0899 | 0.0239             |
| $\{\mathbf{U}\}$ , full                   | 0.8848  | 0.8863  | 0.8835  | 0.0012             |
| $\{\mathbf{U}\}$ , mid                    | 0.8136  | 0.8165  | 0.8090  | 0.0022             |
| $\{H, T\}$ , full                         | 0.7328  | 0.7415  | 0.7194  | 0.0064             |
| $\{H, T\}$ , mid                          | 0.6235  | 0.6416  | 0.6052  | 0.0107             |
| $\{H, \mathbf{U}\}$ , full                | 0.9267  | 0.9493  | 0.9078  | 0.0152             |
| $\{H, \mathbf{U}\}$ , mid                 | 0.8804  | 0.9202  | 0.8493  | 0.0263             |
| $\{\mathbf{U}, T\}$ , full                | 0.9065  | 0.9087  | 0.9034  | 0.0016             |
| $\{\mathbf{U}, T\}$ , mid                 | 0.8458  | 0.8495  | 0.8422  | 0.0025             |
| $\{U\}$ , full                            | 0.6627  | 0.6696  | 0.6521  | 0.0047             |
| $\{U\}$ , mid                             | 0.4800  | 0.4932  | 0.4646  | 0.0080             |
| $\{V\}$ , full                            | 0.7320  | 0.7351  | 0.7290  | 0.0019             |
| $\{V\}$ , mid                             | 0.6030  | 0.6074  | 0.5990  | 0.0028             |
| $\{H, \bar{T}^{25}\}$ , full              | 0.7309  | 0.7434  | 0.7199  | 0.0073             |
| $\{H, \bar{T}^{25}\}$ , mid               | 0.6231  | 0.6416  | 0.6064  | 0.0106             |
| $\{H, \bar{T}^{124}\}$ , full             | 0.7036  | 0.7093  | 0.6957  | 0.0043             |
| $\{H, \bar{T}^{124}\}$ , mid              | 0.5797  | 0.5888  | 0.5654  | 0.0080             |
| $\{\mathbf{U}, \bar{T}^{25}\}$ , full     | 0.9050  | 0.9078  | 0.9008  | 0.0020             |
| $\{\mathbf{U}, \bar{T}^{25}\}$ , mid      | 0.8432  | 0.8477  | 0.8373  | 0.0031             |
| $\{\mathbf{U}, \bar{T}^{124}\}$ , full    | 0.8941  | 0.8956  | 0.8914  | 0.0012             |
| $\{\mathbf{U}, \bar{T}^{124}\}$ , mid     | 0.8249  | 0.8267  | 0.8201  | 0.0018             |
| $\{H, \mathbf{U}, \bar{T}^{25}\}$ , full  | 0.9350  | 0.9484  | 0.9220  | 0.0082             |
| $\{H, \mathbf{U}, \bar{T}^{25}\}$ , mid   | 0.8964  | 0.9189  | 0.8736  | 0.0141             |
| $\{H, \mathbf{U}, \bar{T}^{124}\}$ , full | 0.9315  | 0.9482  | 0.9038  | 0.0155             |
| $\{H, \mathbf{U}, \bar{T}^{124}\}$ , mid  | 0.8903  | 0.9192  | 0.8451  | 0.0257             |
